# Supplementary material for: Two-neutron knockout as a probe of the composition of states in $^{22}$Mg, $^{23}$Al, and $^{24}$Si
Source: arXiv:2002.11839 source file (2020-02-26)
Supplement: Supplementary file 1 [file 2n_knockout_suppl.pdf]

## $L$ Content of Two-Neutron Knockout Overlaps with $^{22}$Mg $2^+$ Final States

This supplementary material clarifies the total orbital angular momentum $L$ ($\vec{L} = \vec{\ell}_1 + \vec{\ell}_2$) content of the two-nucleon overlaps, as expressed by the two-nucleon amplitudes (TNAs). The coupled $jj$-basis TNAs presented in Table I of the text of the Physical Review C Rapid Communication are transformed to the $LS$-basis, since it is the $L$ content that drives the shapes and widths of the longitudinal momentum distributions of the partial cross sections – the smaller $L$ components leading to narrower momentum distributions, see e.g. Refs. [1, 2]. In order to simplify and clarify this $L$ composition, by reducing the number of contributing amplitudes, here we will neglect the small differences between the radial wave functions of the $1d_{5/2}$ and $1d_{3/2}$ $sd$-shell, spin-orbit doublet orbitals. This approximation is very minor but is not made in the full calculations of the Rapid Communication. The shell-model (SM) two-nucleon overlap in the neutron-proton basis and the usual $jj$-coupling scheme, for population of a final state $\Phi_{J_f M_f}(A-2)$ following two-nucleon removal from the projectile state $\Psi_{J_i M_i}(A-2,1,2)$, is [1]

$$\langle \Phi_{J_f M_f}(A-2)|\Psi_{J_i M_i}(A-2,1,2)\rangle = \sum_{I\mu}(I\mu J_f M_f|J_i M_i) \sum_{\alpha} C_\alpha^I\, [\,\overline{\psi_{\beta_1}(1)\otimes\psi_{\beta_2}(2)}\,]_{I\mu}\,. \tag{1}$$

Here $I$ is the transferred angular momentum and $C_\alpha^I \equiv C_\alpha^{(J_i J_f)I}$ the $jj$-coupled TNA, where the label $\alpha \equiv [\beta_1, \beta_2]$, with $\beta \equiv n\ell j$, identifies the single-particle orbitals of the knocked-out nucleon pair. Expressed (exactly) in $LS$-coupling, the antisymmetrized two-nucleon wave function in Eq. (1) is, see Eqs. (2–4) of Ref. [2],

$$\sum_\alpha C_\alpha^I[\,\overline{\psi_{\beta_1}(1)\otimes\psi_{\beta_2}(2)}\,]_{I\mu} = \sum_\alpha D_\alpha \sum_{\substack{L\Lambda S\Sigma\\ \lambda_1\lambda_2}} (\ell_1\lambda_1\ell_2\lambda_2|L\Lambda)(L\Lambda S\Sigma|I\mu)\,\chi_{S\Sigma}(1,2)$$
$$\times\, \mathfrak{C}^I_{\alpha LS}[\psi^{\lambda_1}_{\beta_1}(\vec{r}_1)\psi^{\lambda_2}_{\beta_2}(\vec{r}_2) - (-)^{S+1}\psi^{\lambda_1}_{\beta_1}(\vec{r}_2)\psi^{\lambda_2}_{\beta_2}(\vec{r}_1)] \tag{2}$$

where the $jj$-basis normalisation constant is $D_\alpha = 1/\sqrt{2(1+\delta_{\beta_1\beta_2})}$, $\psi^\lambda_\beta(\vec{r}_i) = u_\beta(r_i)Y_{\ell\lambda}(\hat{\vec{r}}_i)$, and

$$\mathfrak{C}^I_{\alpha LS} = \hat{j}_1\,\hat{j}_2\,\hat{L}\,\hat{S} \begin{Bmatrix} \ell_1 & s & j_1 \\ \ell_2 & s & j_2 \\ L & S & I \end{Bmatrix} C^I_\alpha\,, \tag{3}$$

and $s = 1/2$, the nucleon spin. If we now consider the knockout of neutrons from the $2s_{1/2}$ and $1d_j$ $sd$-shell orbitals and, as stated above, also neglect the small difference in the radial wave functions of the $1d_{5/2}$ and $1d_{3/2}$ spin-orbit doublet, then we can add the contributions from (a) the $[1d_j, 2s_{1/2}]$, and (b) the $[1d_{5/2}, 1d_j]$ and $[1d_{3/2}, 1d_{3/2}]$ TNAs. In this limit, $\psi_{\ell\lambda}(\vec{r}_i) = u_\ell(r_i)Y_{\ell\lambda}(\hat{\vec{r}}_i)$ and Eq. (2) can be rewritten

$$\sum_\alpha C_\alpha^I[\,\overline{\psi_{\beta_1}(1)\otimes\psi_{\beta_2}(2)}\,]_{I\mu} \equiv \sum_{\ell_1\ell_2 LS} D_{\ell_1\ell_2} \sum_{\lambda_1\lambda_2\Lambda\Sigma} (\ell_1\lambda_1\ell_2\lambda_2|L\Lambda)(L\Lambda S\Sigma|I\mu)\,\chi_{S\Sigma}(1,2)$$
$$\times\, C^I(\ell_1,\ell_2,LS)\,[\psi_{\ell_1\lambda_1}(\vec{r}_1)\psi_{\ell_2\lambda_2}(\vec{r}_2) - (-)^{S+1}\psi_{\ell_1\lambda_1}(\vec{r}_2)\psi_{\ell_2\lambda_2}(\vec{r}_1)]\,, \tag{4}$$

where now

$$C^I(\ell_1,\ell_2,LS) = \sum_\alpha D_\alpha\,\mathfrak{C}^I_{\alpha LS}/D_{\ell_1\ell_2} \tag{5}$$

with normalization constants $D_{\ell_1\ell_2} = 1/\sqrt{2(1+\delta_{\ell_1\ell_2})}$. The $L$ content of the overlaps is thus contained in the TNA $C^I(\ell_1,\ell_2,LS)$. For the case of two-neutron removal from $^{24}$Mg, where $J_i = 0$, then of course $I$ is unique and equal to the spin of the final state, $J = J_f$. These $LS$ TNAs for the first three $2^+$ states in $^{22}$Mg are tabulated in Table I, below. It is seen that the $L = 1$ component, $C^2(2,2,11)$, originating from the three $\ell_1 = \ell_2 = 2$ TNAs, is significantly larger than the $L = 2$ terms for the $2^+_1$ state, is comparable with the larger $L = 2$ terms for the $2^+_2$ state, and is very small in the case of the $2^+_3$ state. These different $LS$ terms contribute incoherently to the two-nucleon density and major parts of the partial cross sections [2].


[1] E. C. Simpson, J. A. Tostevin, D. Bazin, and A. Gade, Phys. Rev. C **79**, 064621 (2009).

[2] E. C. Simpson and J. A. Tostevin, Phys. Rev. C **82**, 044616 (2010).

TABLE I. $LS$-decomposed TNAs $C^I(\ell_1, \ell_2, LS)$, of Eq. (5), calculated from the USD interaction $jj$-coupled TNAs for the first three $2^+$ states in $^{22}$Mg populated in two-neutron knockout. Since $J_i = 0$, $I = 2$.

| $I^\pi$ | (2,2,11) | (2,2,20) | (2,0,20) | (2,0,21) | (2,2,31) |
|---|---|---|---|---|---|
| $2_1^+$ | -0.316 | 0.127 | -0.033 | -0.070 | -0.134 |
| $2_2^+$ | -0.654 | -0.438 | -0.309 | 0.033 | 0.054 |
| $2_3^+$ | -0.006 | 0.350 | 0.366 | 0.148 | -0.022 |
